# Supplementary material for: Computational TIRF enables optical sectioning beyond the evanescent field for widefield fluorescence microscopy
Source: arXiv:2511.06853 source file (2026-01-23)
Supplement: Supplementary file 1 [file SI_for_ETNet.pdf]

## **Supplementary Information for**

Deep learning EPI-TIRF cross-modality enables background subtraction and axial super-resolution for widefield fluorescence microscopy

Qiushi Li, Celi Lou, Yunqing Tang\*, Luru Dai\* and et al.

Email: tang@ucas.ac.cn; dai@ucas.ac.cn;

## Contents

|                                                                                               |    |
|-----------------------------------------------------------------------------------------------|----|
| Supplementary Figures .....                                                                   | 3  |
| Supplementary Tables .....                                                                    | 5  |
| Supplementary Note 1. Implementation of background-removal and deconvolution algorithms ..... | 6  |
| Supplementary Note 1.1 Dark Sectioning .....                                                  | 6  |
| Supplementary Note 1.2 BF-SIM (background removal part) .....                                 | 6  |
| Supplementary Note 1.3 WBNS .....                                                             | 7  |
| Supplementary Note 1.4 Sparse Deconvolution .....                                             | 7  |
| Supplementary Note 1.5 RL deconvolution.....                                                  | 8  |
| Supplementary Note 2. Combination of ETNet and Sparse Deconvolution .....                     | 9  |
| Supplementary Note 3. Implementation of 3D reconstruction method .....                        | 11 |
| Supplementary Note 3.1 DW .....                                                               | 11 |
| Supplementary Note 3.2 Self-Net.....                                                          | 11 |
| Supplementary Note 3.3 UniFMIR.....                                                           | 11 |
| Supplementary Note 4. Three-dimensional reconstruction with limited layers.....               | 12 |
| Supplementary Note 5. Details on WF and confocal image registration.....                      | 14 |
| Supplementary Note 6. Details on training ET2dNet for ET3dNet.....                            | 16 |
| References.....                                                                               | 18 |

## Supplementary Figures

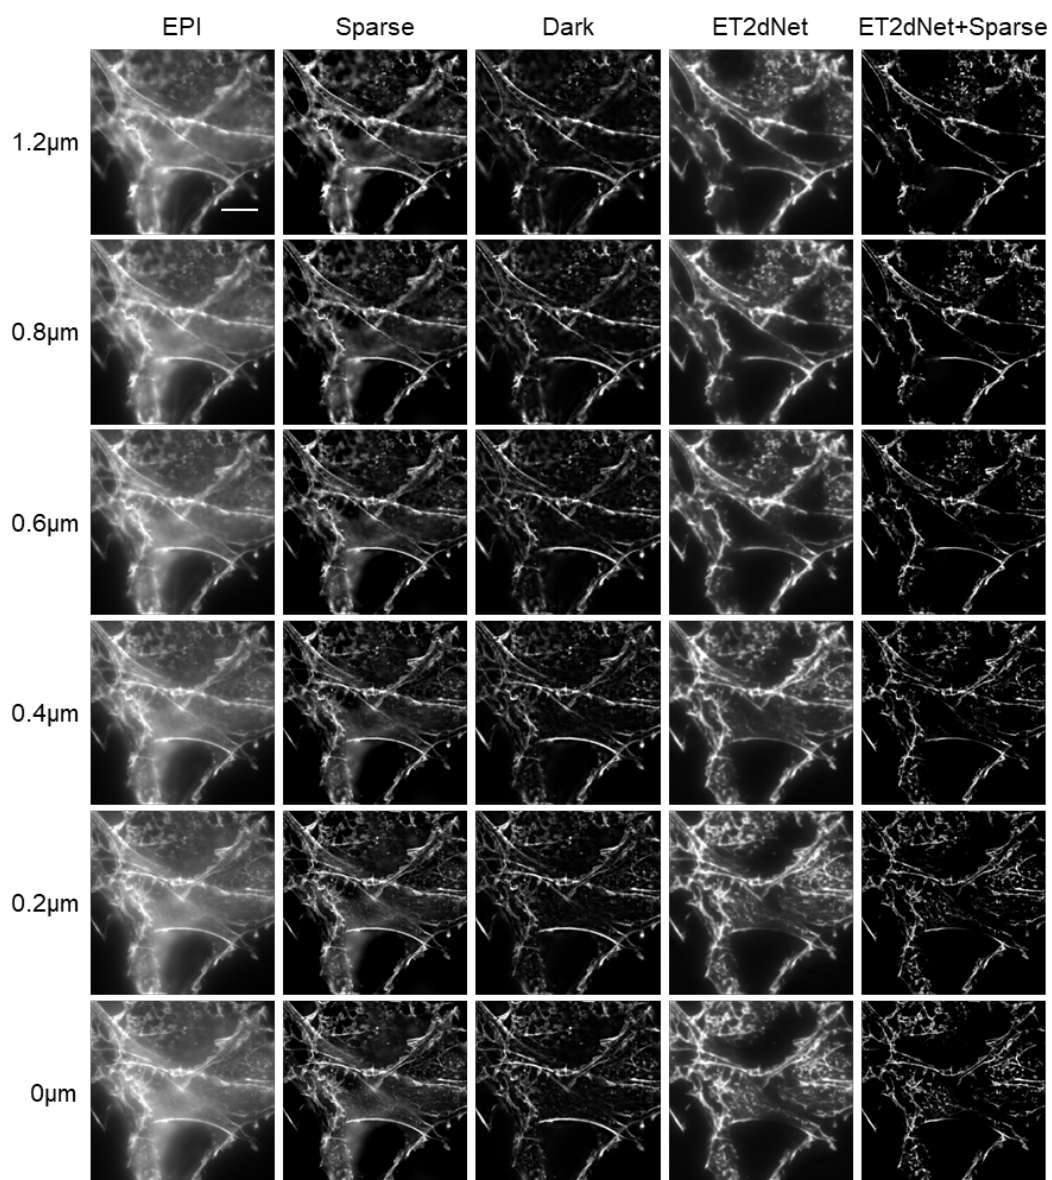

**Fig. S1** The full image stack corresponding to Fig. 1d in the main text. Scale bar: 10 $\mu$ m.

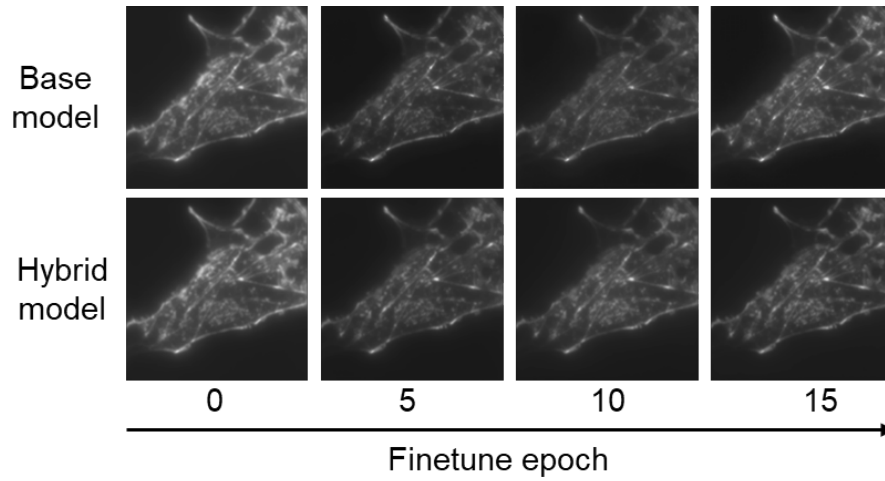

**Fig. S2** The full images corresponding to Fig. 2c in the main text. Scale bar: 10 $\mu$ m.

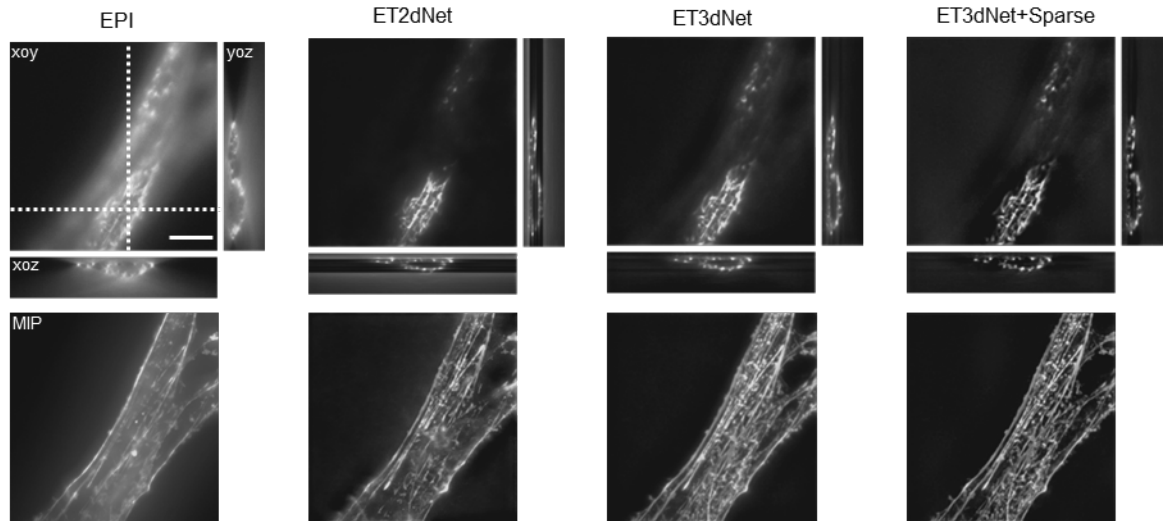

**Fig. S3** A representative example of C6 cell to illustrate the artifact of discontinues intensity distribution along z-direction for directly applying ET2dNet on WF image stack, and corresponding artifact-reduced result for ET3dNet. Scale bar: 10 $\mu$ m.

## Supplementary Tables

**Table 1 The imaging details of figures in the main text and the extended data.**

| Figure               | Sample             | Origin                                      | Modality    | Excitation Wavelength(nm) and corresponding fluorescent label                 | NA   | Magnification | Pixel Size(nm)             |
|----------------------|--------------------|---------------------------------------------|-------------|-------------------------------------------------------------------------------|------|---------------|----------------------------|
| Fig.1 c,d            | C6 cell            | EPI-TIRF microscope with laser illumination | EPI TIRF    | 638 (Alexa Fluor™ 635 Phalloidin)                                             | 1.5  | 60            | 97.5(lateral)              |
| Fig.1 f              | Human brain tissue | Data in Ref. <sup>1</sup>                   | WF confocal | 580(Alexa Fluor 555)                                                          | 1.45 | 60            | 107.9(lateral )            |
| Fig.2 a,c            | C6 cell            | EPI-TIRF microscope with laser illumination | EPI TIRF    | 638(Alexa Fluor™ 635 Phalloidin)                                              | 1.5  | 100           | 80(lateral)                |
| Fig.2 e              | Human brain tissue | Data in Ref. <sup>1</sup>                   | WF confocal | 580(Alexa Fluor 555)                                                          | 1.45 | 100           | 65(lateral)                |
| Fig.3 b              | C6 cell            | EPI-TIRF microscope with LED illumination   | EPI         | 638(Alexa Fluor™ 635 Phalloidin)                                              | 1.5  | 60            | 97.5(lateral) 200(axial)   |
| Fig.3 c              | C6 cell            | EPI-TIRF microscope with LED illumination   | EPI         | 638(Alexa Fluor™ 635 Phalloidin) 488(Alexa Fluor™ 488 WGA) 405(Hoechst 33258) | 1.5  | 60            | 97.5(lateral) 200(axial)   |
| Fig.3 d              | Human brain tissue | Data in Ref. <sup>1</sup>                   | WF confocal | 580(Alexa Fluor 555)                                                          | 1.4  | 60            | 107.9(lateral ) 200(axial) |
| Extended Data Fig. 1 | U87 cell           | EPI-TIRF microscope with laser illumination | EPI TIRF    | 638 (Alexa Fluor™ 635 Phalloidin)                                             | 1.5  | 60            | 97.5(lateral)              |
| Extended Data Fig. 2 | C6 cell            | EPI-TIRF microscope with laser illumination | EPI TIRF    | 638 (Alexa Fluor™ 635 Phalloidin)                                             | 1.5  | 60            | 97.5(lateral)              |

## Supplementary Note 1. Implementation of background-removal and deconvolution algorithms

In this section, we give a brief introduction to each background-removal and deconvolution algorithms mentioned in the main text, with corresponding implementation details.

### Supplementary Note 1.1 Dark Sectioning

The Dark Sectioning<sup>2</sup> leverages dark channel priors to discriminate between in-focus and out-of-focus signals by integrating point spread function (PSF) constraints into its algorithm. For a given image  $I(x, y)$ , the dark channel is defined as:

$$\text{dark}[I(x, y)] = \min I(x - \Delta x/2 : x + \Delta x/2, y - \Delta y/2 : y + \Delta y/2),$$

where  $\Delta x$  and  $\Delta y$  denote the block size of dark channel determined by the PSF. The reconstruction procedure is mathematically expressed through the following operations,

$$\begin{aligned} J(x, y) &= J_{Lo}(x, y) + J_{Hi}(x, y) \\ J_{Hi}(x, y) &= HI\{I(x, y)\} \\ J_{Lo}(x, y) &= \frac{Lo\{I(x, y)\} - \text{dark}\left[\frac{Lo\{I(x, y)\}}{EL\{I(x, y)\}}\right] EL\{I(x, y)\}}{1 - \text{dark}\left[\frac{Lo\{I(x, y)\}}{EL\{I(x, y)\}}\right]}. \end{aligned}$$

Here  $J(x, y)$  and  $I(x, y)$  represent the reconstructed and raw image, respectively.  $Lo\{\}$ ,  $HI\{\}$ , and  $EL\{\}$  represent the low-pass, high-pass, and extreme low-pass filter, respectively. For implementation, we used the author suggested parameters, since we found fine-tuning the parameters (e.g., EL) gave similar results.

### Supplementary Note 1.2 BF-SIM (background removal part)

The Background Filtered SIM (BF-SIM) algorithm<sup>3</sup> suppresses out-of-focus background in SIM imaging. Its theoretical foundation relies on a core hypothesis:

$$[g(\mathbf{r}, z_{in}) \cdot I(\mathbf{r})] \otimes h(\mathbf{r}, z_{out}) \approx [g(\mathbf{r}, z_{out}) \cdot I(\mathbf{r})] \otimes h(\mathbf{r}, z_{out}),$$

where  $g(\mathbf{r}, z_{in})$  and  $g(\mathbf{r}, z_{out})$  are the in-focus and out-of-focus ground truth, respectively.  $h(\mathbf{r}, z_{out})$  represents the PSFs with the range out-of-focus  $z_{out}$ .  $I(\mathbf{r})$  is the illumination pattern.  $\otimes$  is the convolution operator. Assuming uniform illumination ( $I(\mathbf{r}) = 1$ ), this hypothesis extends to WF imaging, yielding the BF reconstruction

$$d_{in}(\mathbf{r}) = d(\mathbf{r}) - \text{iFt}\left\{D(k) \cdot \frac{\text{Ft}\{d(\mathbf{r})\}}{\text{Ft}\{h(\mathbf{r}, z_{in})\} + \text{Ft}\{h(\mathbf{r}, z_{out})\}}\right\},$$

where  $d(\mathbf{r})$  and  $d_{in}(\mathbf{r})$  represent the raw image and in-focus image respectively.  $h(\mathbf{r}, z_{in})$  represents the PSFs within the range in-focus  $z_{in}$ .  $\text{Ft}\{\}$  and  $\text{iFt}\{\}$  denotes

Fourier and inverse Fourier transform, respectively. For implementation, we regarded the PSF within the range of  $(-0.4 \mu m, 0.4 \mu m)$  as  $h(\mathbf{r}, z_{in})$  and that in the range of  $(-4 \mu m, -0.4 \mu m)$  and  $(0.4 \mu m, 4 \mu m)$  as  $h(\mathbf{r}, z_{out})$ , as the author suggested.

### Supplementary Note 1.3 WBNS

The wavelet-based background and noise subtraction (WBNS) algorithm<sup>4</sup> employs the Haar wavelet transform to simultaneously suppress low-frequency background and high-frequency noise. The processing steps are mathematically defined as follows:

$$J(x, y) = I(x, y) - WBS(x, y) - noise(x, y)$$

$$WBS(x, y) = WT^{-1}\{WT^{-1}\{WT^{-1}\{Lo(WT\{Lo(WT\{Lo(WT\{I(x, y)\})\})\})\})\})\}$$

$$noise(x, y) = WT^{-1}\{Hi(WT\{I(x, y)\})\}$$

Here  $J(x, y)$  and  $I(x, y)$  represent the reconstructed and raw image, respectively.  $WT\{\}$  and  $WT^{-1}\{\}$  represent the Haar wavelet transform and inverse Haar wavelet transform, respectively.  $Lo\{\}$  represents a low-pass filter, which sets the detail coefficients to zero.  $Hi\{\}$  represents a high-pass filter, which sets the approximation coefficients to one. For implementation we used the author suggested parameters, since we found finetuning the parameters gave similar results.

### Supplementary Note 1.4 Sparse Deconvolution

The Sparse Deconvolution<sup>5</sup> incorporates sparsity prior through explicit regularization within the minimization framework:

$$\arg \min_{x, b} \left\{ \frac{\lambda}{2} \|\mathbf{f} - \mathbf{b} - \mathbf{A}\mathbf{x}\|_2^2 + R_{Hessian}(\mathbf{x}) + \lambda_{L1} \|\mathbf{x}\|_1 \right\},$$

where  $\|\mathbf{f} - \mathbf{b} - \mathbf{A}\mathbf{x}\|_2^2$  represents the residual between the recovered image  $\mathbf{x}$  and the raw image  $\mathbf{f}$ .  $\mathbf{A}$  denotes the convolution operator with PSF.  $\mathbf{b}$  represents the background.  $R_{Hessian}(\mathbf{x})$  and  $\|\mathbf{x}\|_1$  are regularization terms corresponding to continuity and sparsity prior, respectively. Background estimation employs an iterative wavelet-based procedure:

$$\mathbf{b}_n = WT^{-1}\{Lo(WT\{I_n\})\}$$

$$I_{n+1} = \min[I_0, \sqrt{I_n}/2 + \mathbf{b}_n]$$

Here,  $WT\{\}$  and  $WT^{-1}\{\}$  represent the wavelet transform and the inverse wavelet transform, respectively.  $Lo()$  represents the lowest frequency wavelet band.  $I_n$  and  $\mathbf{b}_n$  represent the image and background, respectively.  $I_0$  represents the raw image  $\mathbf{f}$ . Convergence typically occurs within three iterations. For the complete implementation of Sparse Deconvolution, we set fidelity = 300, sparsity = 3, and iterations = 100.

### Supplementary Note 1.5 RL deconvolution

The famous Richardson and Lucy (RL)<sup>6</sup> deconvolution follows the iteration:

$$\mathbf{x}_{n+1} = \mathbf{x}_n \left( \mathbf{A}^{-1} \frac{\mathbf{f}}{\mathbf{A}\mathbf{x}_n} \right),$$

where  $\mathbf{x}_n$  represents the  $n$ th reconstruction,  $\mathbf{f}$  represents the raw image.  $\mathbf{A}$  denotes the convolution operator with PSF.  $\mathbf{A}^{-1}$  is the conjugate of  $\mathbf{A}$ . For implementation, we set iterations = 10.

## Supplementary Note 2. Combination of ETNet and Sparse

### Deconvolution

The lateral resolution of fake GT generated by ETNet (2d or 3d) exhibits limited improvement compared to raw images, since the ETNet was not specifically optimized for deconvolution. Although a self-supervised loss function (fake GT \* PSF = TIRF) was employed, the ill-posed nature of the problem allows solutions to reside in an excessively large solution space around the real GT. A possible way is to establish a loss function between fake GT and deconvolved TIRF results, inspired by the framework of zero-shot network<sup>7</sup>. Another possible way is to carefully finetune both network architecture and regularization terms in loss function, referring to Deep Image Prior technique<sup>8</sup>. Notably, direct integration of ETNet with SOTA deconvolution methods further enhances lateral resolution, as demonstrated in the main text. Below we give the implementation details.

For ET2dNet, Sparse deconvolution was applied with optimized parameters (fidelity = 300, sparsity = 3). Iterations of 100 and 20 yielded nearly identical results (this consistency was validated across all tested samples as shown in Fig. S4), justifying the selection of 100 iterations. For ET3dNet, Sparse Deconvolution was applied to each axial slice  $I(x, y, z)$ , yielding  $I'(x, y, z)$ . To ensure intensity conservation, the final output was normalized as,

$$I''(x, y, z) = I'(x, y, z) \times \frac{\sum_{x,y} I'(x, y, z)}{\sum_{x,y} I(x, y, z)}.$$

Deconvolution parameters were consistent (fidelity = 300, sparsity = 3, iterations = 100).

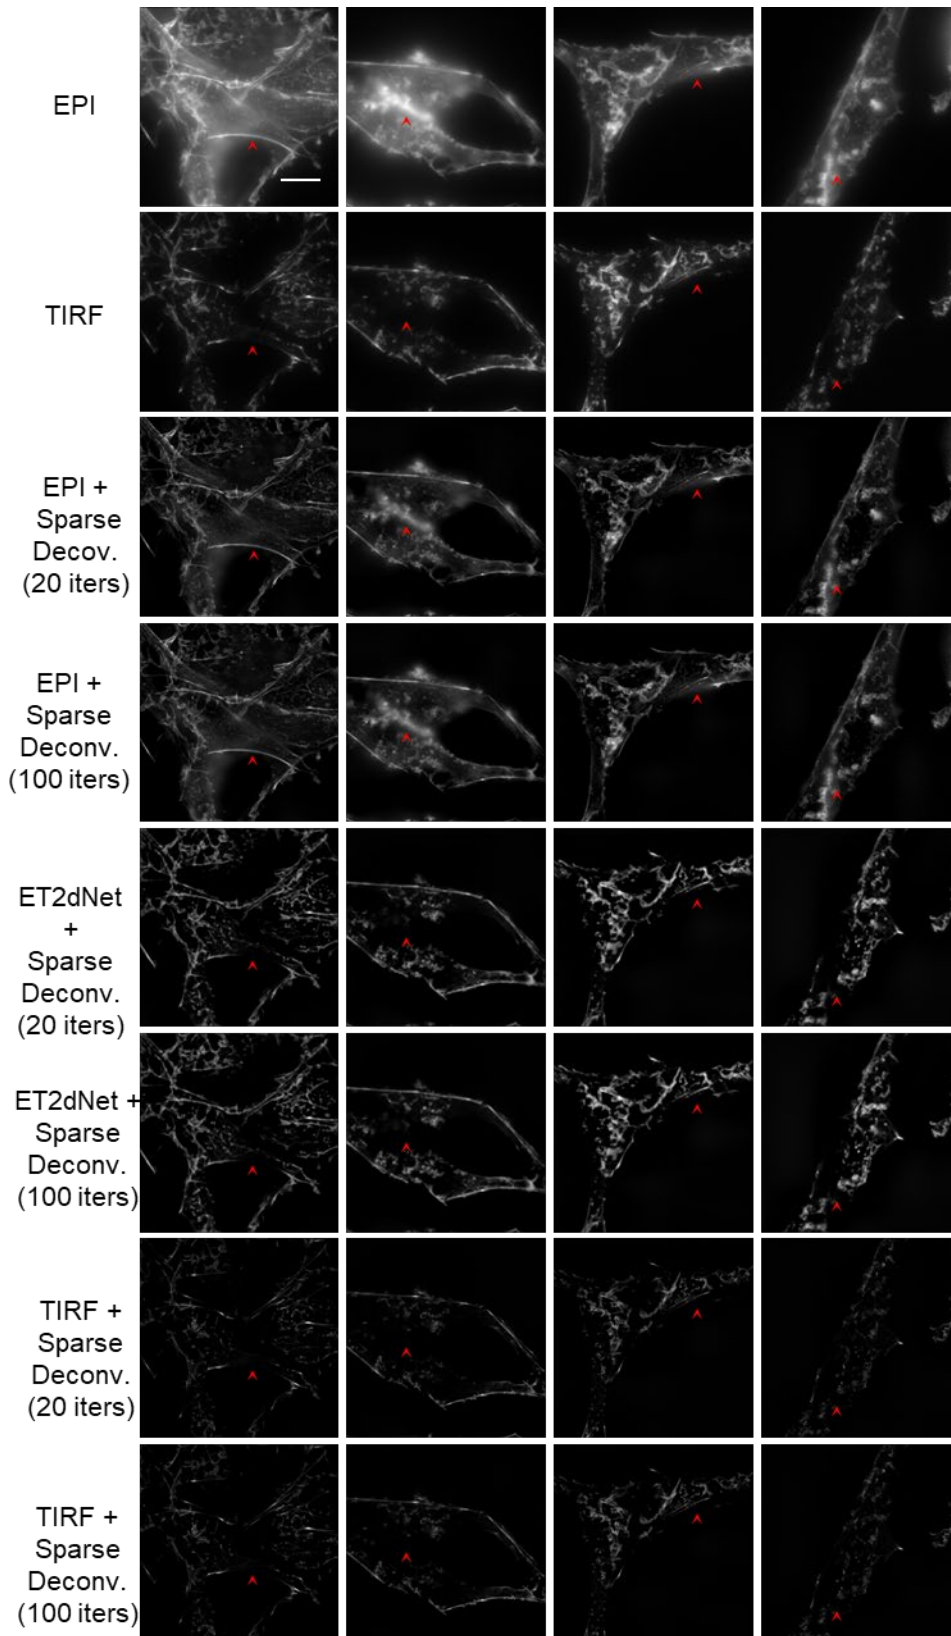

**Fig. S4 Representative examples of Sparse Deconvolution for 20 and 100 iterations, which yielded nearly identical results. Scale bar: 10 $\mu$ m.**

### **Supplementary Note 3. Implementation of 3D reconstruction method**

In this section, we give a brief introduction to each 3D reconstruction algorithms mentioned in the main text, with corresponding implementation details.

#### **Supplementary Note 3.1 DW**

Deconvolf (DW) is an easy-to-operate and computationally efficient deconvolution software<sup>1</sup>. For implementation, we used the PSFs generated by DW and set iterations = 100.

#### **Supplementary Note 3.2 Self-Net**

Self-Net is a deep learning framework designed for high-fidelity isotropic resolution restoration in volumetric fluorescence microscopy imaging, which only needs one image stack as input by employing self-learning strategy<sup>9</sup>. In our implementation, we adopted the original network architecture and hyperparameters, substituting only the input image data for validation.

#### **Supplementary Note 3.3 UniFMIR**

UniFMIR is a unified deep learning model for fluorescence microscopy image restoration, capable of addressing diverse degradation types<sup>10</sup>. For our evaluation, we deployed the model locally via its web interface and performed inference using our custom microscopy datasets.

## **Supplementary Note 4. Three-dimensional reconstruction with**

### **limited layers**

The 3D reconstruction of real-time imaging for WF tomography faces a fundamental challenge, where the requirement of sufficient slices to give faithful reconstruction slows down the imaging speed. In this section, we investigate the dependence of background removal capability of DW on stack size, as shown in Fig. S5. Here the DW deconvolution is performed on image stacks with growing size, while the central layer is same for each stack.

The DW deconvolution was performed on a C6 cell stack with different size of slices (of 3, 5, 7, 9, 11), while the results of central layer are shown in Fig. S5b. Note that, the central layer is exactly the sample shown in Fig. 1c in the main text. Then we analyzed the intensity distribution along the red lines in Fig. S5b, as shown in Fig. S5d, which indicated that for larger stack the DW deconvolution gave more faithful results with less background. Then another example of C6 cell stack with more slices (of 3,13,23,33,43) were analyzed, as shown in Fig. S5c. Visually, the background removal capability of DW was more efficient for stacks with more slices, which is also supported by the profiles of intensity distribution along red lines (Fig. S5e). All these results consistently indicated that DW deconvolution performs better when the GT is completely enclosed within the WF stack, and DW results show obvious backgrounds (or artifacts) with limited layers.

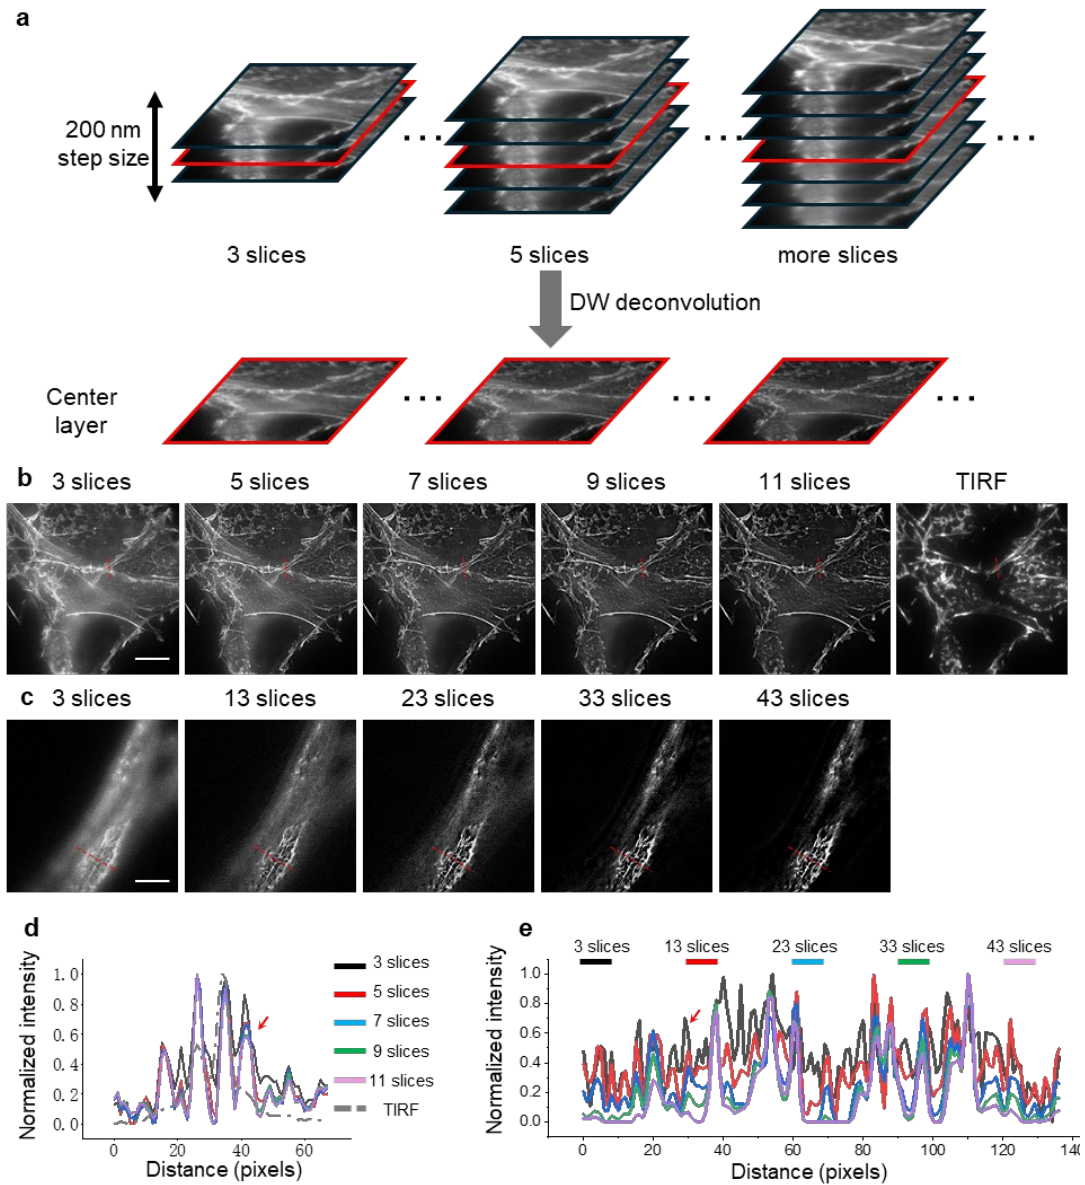

**Fig. S5 The dependence of background removal capability of DW on stack size. a,** illustration of the implementation of DW deconvolution on stacks with different size. **b, c,** center slices of two representative image stacks of F-actin labeled C6 cell, **d, e,** corresponding profile of normalized intensity along red lines in (d) and (e). Scale bar: 10 $\mu$ m.

## Supplementary Note 5. Details on WF and confocal image

### registration

Since the WF and confocal image pairs (Fig. 1f, 2e, 3d in main text) were acquired using two distinct microscopy systems (see Ref.<sup>1</sup> for more details), spatial alignment was necessary to enable comparative analysis. To achieve this, we performed image registration by manually selecting corresponding feature points and computing an affine transformation matrix. The registration results are presented in Fig. S6, which displays (from left to right): the raw WF image, the registered confocal image, and a composite pseudo-color overlay of the aligned channels.

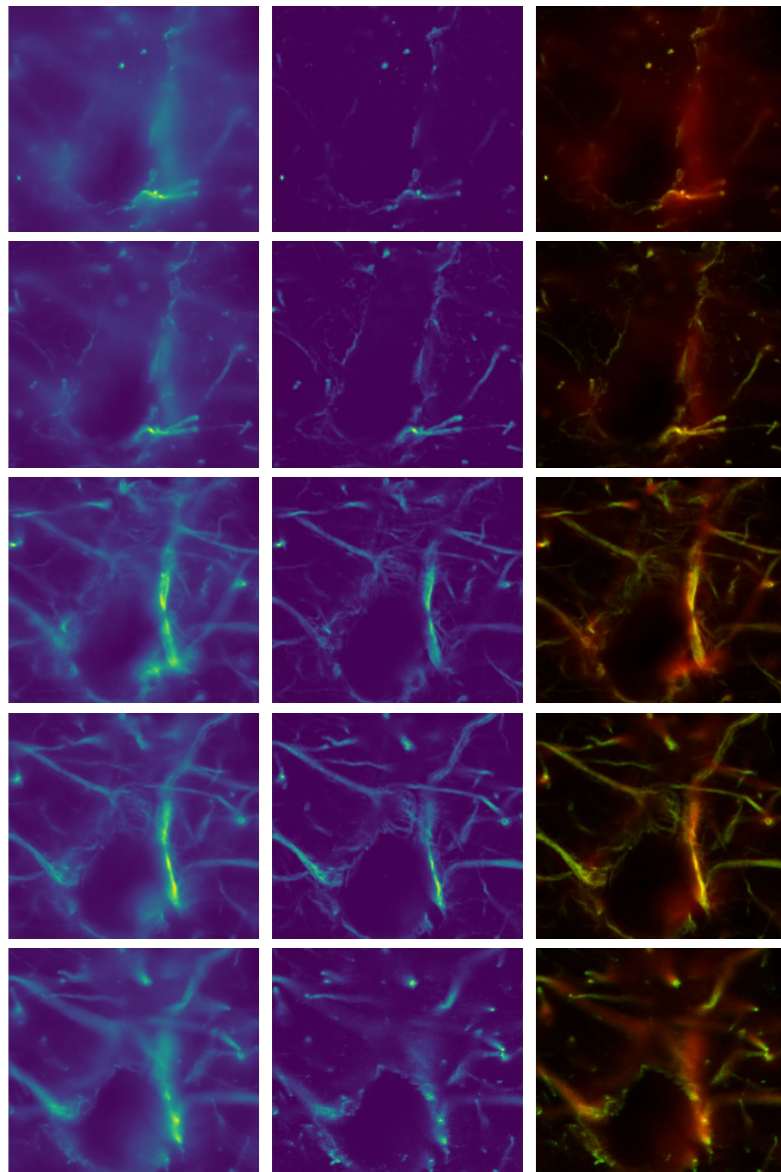

**Fig. S6 Representative registration results of WF and confocal image pairs.** WF images (first column), registered confocal images (second column), and the composite pseudo-color overlay (third column).

## Supplementary Note 6. Details on training ET2dNet for ET3dNet

Note that ET2dNet was trained on single 2D images and did not yield optimal results when directly applied to full 3D stacks. During training, we prepared a representative 3D stack and, at every fifth epoch, processed this stack to evaluate the xz cross-sections (see Fig. S7). Both the cross-sectional results and corresponding model parameters were saved. Upon completion of training, we manually selected the model exhibiting the best performance on the xz cross-sections, which was subsequently used as the teacher network for training ET3dNet.

Fig. S7 illustrates the evolution of xz-plane reconstructions from a representative 3D stack processed by ET2dNet at different training stages. The value in the top-left corner of each panel denotes the loss on the test set at that stage, which decreased progressively as training advanced. Despite this, the quality of the xz-plane outputs varied significantly even at similar loss values. The orange box highlights the model checkpoint with the lowest loss, representing the optimal state for processing single-layer images; however, substantial background noise was still apparent in the xz-plane at this point. Therefore, we selected the model checkpoint marked by the green box for ET3dNet training, as it achieved a comparable loss but yielded noticeably cleaner background in the volumetric output.

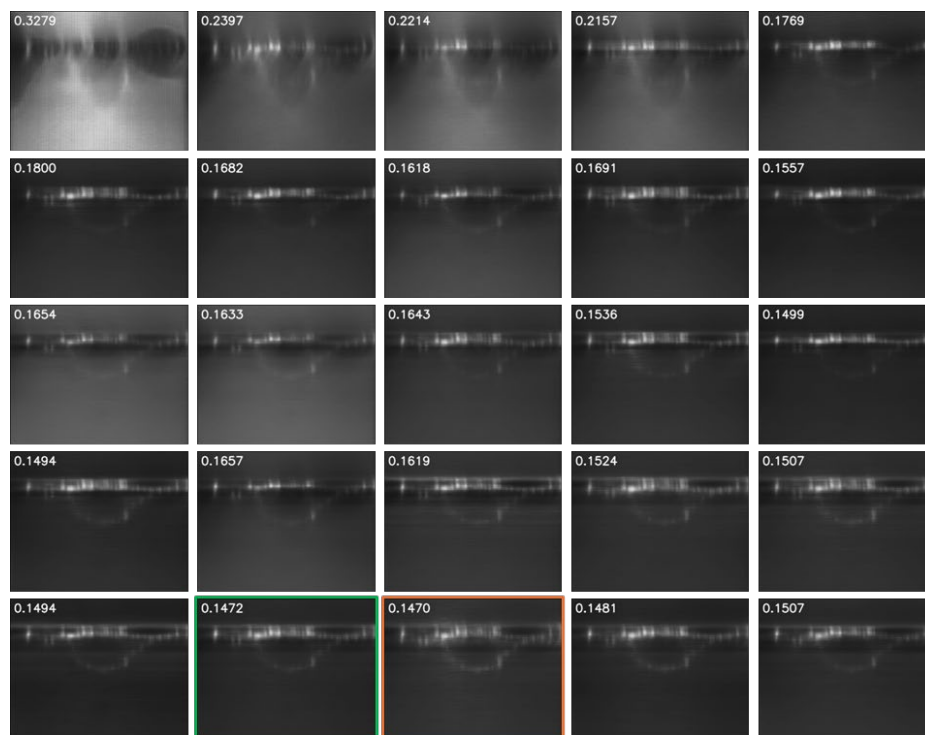

**Fig. S7 Representative xz-plane view from a 3D image stack at every fifth epoch**

**during the training process of ET2dNet.**

## References

1. Wernersson E, Gelali E, Girelli G, et al. Deconvolf enables high-performance deconvolution of widefield fluorescence microscopy images. *Nature Methods*. 2024;21(7):1245-1256.
2. Cao R, Li Y, Zhou Y, et al. Dark-based optical sectioning assists background removal in fluorescence microscopy. *Nature Methods*. 2025;22(6):1299-1310.
3. Mo Y, Wang K, Li L, et al. Quantitative structured illumination microscopy via a physical model-based background filtering algorithm reveals actin dynamics. *Nat Commun*. 2023;14(1):3089.
4. Hüpfel M, Yu. Kobitski A, Zhang W, Nienhaus GU. Wavelet-based background and noise subtraction for fluorescence microscopy images. *Biomedical Optics Express*. 2021;12(2):969-980.
5. Zhao W, Zhao S, Li L, et al. Sparse deconvolution improves the resolution of live-cell super-resolution fluorescence microscopy. *Nat Biotechnol*. 2022;40(4):606-617.
6. Bertero M, Boccacci P, De MoI C. *Introduction to Inverse Problems in Imaging*. 2nd ed. CRC Press; 2021.
7. Qiao C, Zeng Y, Meng Q, et al. Zero-shot learning enables instant denoising and super-resolution in optical fluorescence microscopy. *Nat Commun*. 2024;15(1):4180.
8. Lempitsky V, Vedaldi A, Ulyanov D. Deep Image Prior. In: *2018 IEEE/CVF Conference on Computer Vision and Pattern Recognition*. IEEE; 2018:9446-9454.
9. Ning K, Lu B, Wang X, et al. Deep self-learning enables fast, high-fidelity isotropic resolution restoration for volumetric fluorescence microscopy. *Light Sci Appl*. 2023;12(1):204.
10. Ma C, Tan W, He R, Yan B. Pretraining a foundation model for generalizable fluorescence microscopy-based image restoration. *Nature Methods*. 2024;21(8):1558-1567.
